# Supplementary material for: PoCo: Point Context Cluster for RGBD Indoor Place Recognition
Source: arXiv:2404.02885 source file (2024-12-16)
Supplement: Supplementary file 1 [file appendix.tex]

\begin{figure*}[h!]
  \centering
  \begin{tabular}{ | c | c | c | c | }
    \hline
   \textbf{Query Frames} & \textbf{PoCo} & \textbf{Ground Truth} \\ \hline
    % \textbf{Too similar Geometric structure and matched point cloud doesn't have similar structure}&
    \begin{minipage}{.22\textwidth}
    \includegraphics[width=\linewidth,height=0.7\linewidth]{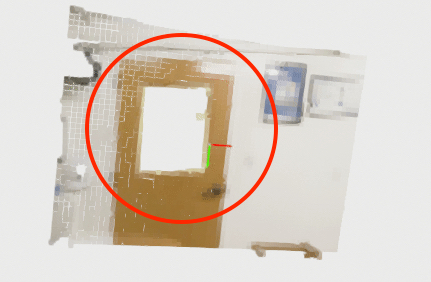}
    \end{minipage}
    &
    \begin{minipage}{.22\textwidth}
      \includegraphics[width=\linewidth,height=0.7\linewidth]{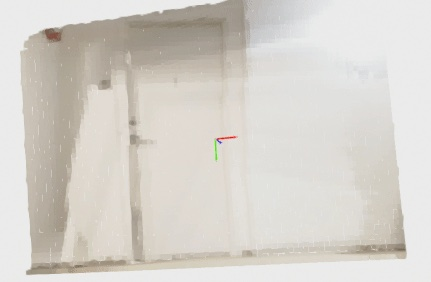}
    \end{minipage}
    & 
    \begin{minipage}{.22\textwidth}
      \includegraphics[width=\linewidth,height=0.7\linewidth]{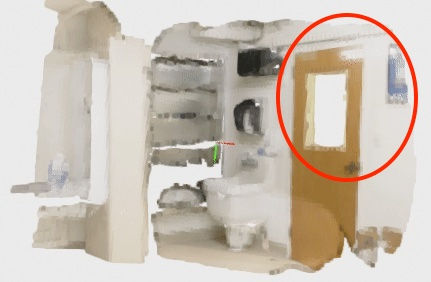}
    \end{minipage}
    
    \\ \hline
    \begin{minipage}{.22\textwidth}
      \includegraphics[width=\linewidth,height=0.7\linewidth]{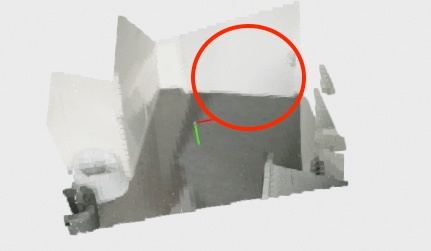}
    \end{minipage}
    &
    \begin{minipage}{.22\textwidth}
      \includegraphics[width=\linewidth,height=0.7\linewidth]{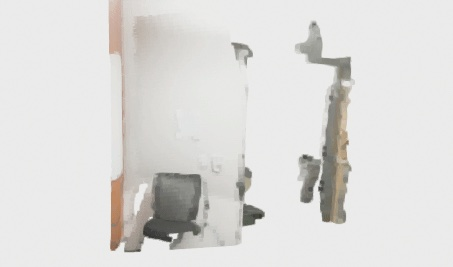}
    \end{minipage}
    & 
    \begin{minipage}{.22\textwidth}
      \includegraphics[width=\linewidth,height=0.7\linewidth]{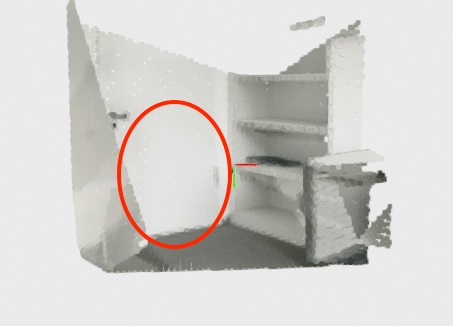}
    \end{minipage}
    
    \\ \hline
  \end{tabular}
  \caption{Corner Cases: If the geometric shape of the wrong match is very similar and the best match has very different scale, as the first row, the model confuses. If the overlapping areas are too flat with single color, the model also cannot perform well.}
  \label{fig:discussion}
\end{figure*}

\section{Supplement}
\label{sec:discussion}

In the experiment, we realized there are several corner cases that the PoCo method cannot fully solve. 
\begin{enumerate}
    \item \textbf{Similar geometric structure with similar scale:} PoCo model explicitly encodes the geometric information that helps a lot in performance, but it also gives some noise to the matching performance. As the first row in Fig. \ref{fig:discussion}, when the doors are too similar and also in the very same scale while the ground truth point cloud has a very different scale and only contains part of the door, the PoCo model confuses in detecting the best matching frame.
    \item \textbf{Overlapping area is too small and not much features:} As the second row in Fig. \ref{fig:discussion}, the overlapping area is only the bottom of the white door, where the overlapping area is very small and the overlapping area is only a white and flat surface. Our PoCo model also struggles in this situation.
\end{enumerate}
